# Supplementary material for: Neural Language Priors
Source: arXiv:1910.03492 source file (2019-10-04)
Supplement: Supplementary file 2 [file appendixA.tex]

\subsection{Appendix: Results with mean-pooling}
\label{subsec:appendixa}

We present our main results with mean pooling on Table \ref{figure:results_mean}, which depicts the performance of our different models across various sentence embedding sizes.

\begin{figure*}[h]
  \centering
    \includegraphics[width=\linewidth]{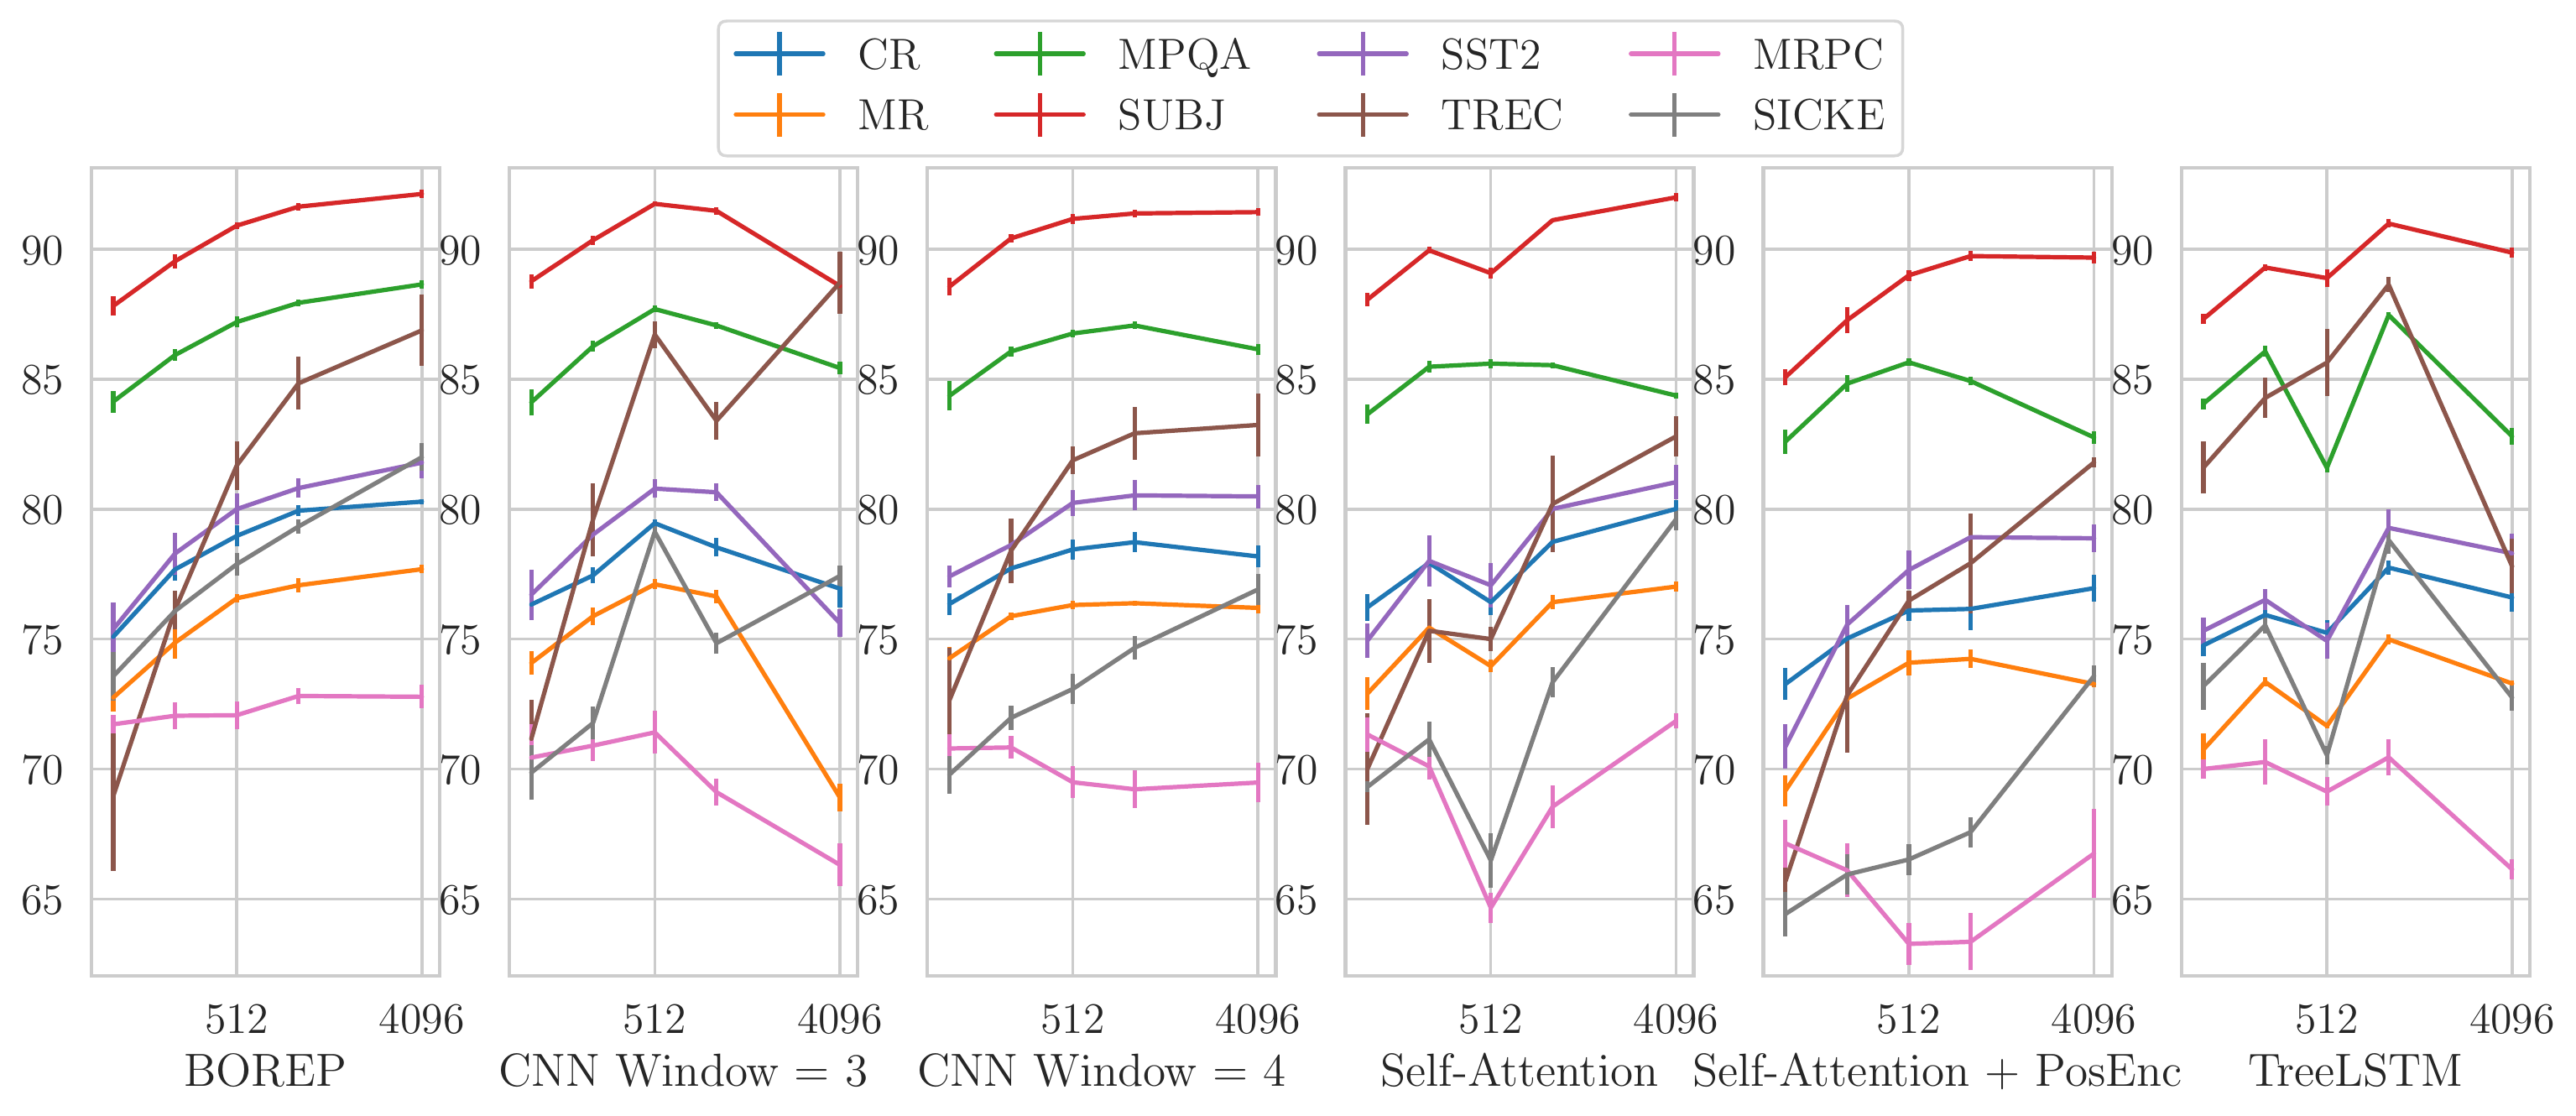}
  \caption{Results with mean-pooling for random \gls{borep}, \gls{cnn} with windows 3 and 4, Tree\gls{lstm} and self-attention with positional encoding. As for max-pooling, this figure shows that every network investigated performs similarly, if not worse, than a simple \gls{borep}, indicating that there is no known prior for sentence embedding.
  It can also be inferred from these results that the self-attention with positional embedding network performs poorly on these downstream task, indicating that this algorithm is a weak prior for sentence embedding.
  Furthermore, the Tree\gls{lstm}, which perform generally well with max-pooling, performs badly with mean-pooling, even on tasks such as TREC, which gives particularly good results with max-pooling.
  Finally, as already suggested in \cite{Conneau2018a}, \gls{lstm}s and its variations perform worse with mean-pooling than with max-pooling. However, for other types of networks, the results on SentEval are relatively independent of the type of pooling.
  \label{figure:results_mean}
  }
\end{figure*}
